# Supplementary material for: First-principles prediction of potentials and space-charge layers in all-solid-state batteries
Source: arXiv:1902.11158 source file (2019-04-02)
Supplement: Supplementary file 1 [file Supplemental_Material.pdf]

# Supplemental Material: First-principles prediction of potentials and space-charge layers in all-solid-state batteries

## S.I. IONIC AND ELECTRONIC PARTS OF OCV

This section contains a more detailed derivation of the separation of the open-circuit voltage into ionic and electronic parts. The cell voltage of an intercalation compound is given by

$$-eV = \tilde{\mu}^c_{e^-} - \tilde{\mu}^a_{e^-}. \tag{S.1}$$

Here $\tilde{\mu}_X$ is electrochemical potential of species $X$: $\tilde{\mu}_X = \mu_X + q_X\phi$, $\mu_X$ is chemical potential of species $X$, $q_X$ is its charge, and $\phi$ is the Galvani (electrostatic) potential. Superscripts $a$ and $c$ indicate the anode and cathode respectively.

$$-eV = \mu^c_{e^-} - \mu^a_{e^-} - e\left(\phi^c - \phi^a\right). \tag{S.2}$$

Since the intercalated species $M^+$ is free to flow throughout the battery, the electrochemical potential $\tilde{\mu}_{M^+}$ must be constant in equilibrium:

$$\tilde{\mu}^a_{M^+} = \tilde{\mu}^c_{M^+}, \tag{S.3}$$

$$\mu^a_{M^+} + e\phi^a = \mu^c_{M^+} + e\phi^c, \tag{S.4}$$

$$-e(\phi^c - \phi^a) = \mu^c_{M^+} - \mu^a_{M^+}. \tag{S.5}$$

Substituting into Eq. S.2,

$$-eV = \mu^c_{e^-} - \mu^a_{e^-} + \mu^c_{M^+} - \mu^a_{M^+}. \tag{S.6}$$

Therefore the cell voltage may be divided into an electronic contribution $V_{e^-}$ and an ionic contribution $V_{M^+}$:

$$-eV_{e^-} = \mu^c_{e^-} - \mu^a_{e^-}, \tag{S.7}$$

$$-eV_{M^+} = \mu^c_{M^+} - \mu^a_{M^+}, \tag{S.8}$$

$$V = V_{e^-} + V_{M^+}. \tag{S.9}$$

## S.II. VACUUM ALIGNMENT METHODOLOGY

In order to calculate ionization potentials and work functions, a supercell is created containing a slab terminated by the chosen surface separated by a vacuum space. Vacuum spacing and slab thickness are chosen to be 15 Å. The planar-average electrostatic potential is calculated, and the shift between the vacuum value and the average bulk value is then used to align the bulk band structure on an absolute energy scale. We partially automate surface generation and analysis using pymatgen [1]. The ionization potential is the position of the valence-band maximum below the vacuum level, and the work function is the position of the Fermi level below the vacuum.

For $LiCoO_2$, the low energy (104) surface is used. The ionization potential is $I = 5.33$ V, and increases to $I = 6.38$ V in $Li_{0.5}CoO_2$. The work function of Li metal (using the (110) surface) is calculated to be 3.14 V. In $SD$-LiPON, the lowest-energy non-polar surface, $(1\bar{1}0)$ gives the vacuum alignment: $I = 5.56$ V.

It is worth noting that these calculated work functions are a surface properties, and using them to obtain bulk band alignments and $V_{e^-}$ is an approximation. However, aligning bands levels to the vacuum using comparable surfaces is common practice when calculating band offsets in semiconductors in circumstances where an explicit interface is difficult (e.g. because of lattice mismatch) [2]. This connection between band offsets and vacuum alignment can be justified with the "model solid" theory [3]. While the validity of this approach is less well tested in the context of battery materials, the lowest-energy surfaces are likely to be most representative of terminations in real devices (in the absence of intentional targeting of a higher-energy surface). So while the Li work function varies from 2.83 to 3.27 V among tested surfaces, and the LiPON ionization potential varies from 4.94 to 5.56 V, we believe our approximation has better uncertainty than this range of values would indicate. Additionally, our approach has the advantage of being systematic. All surfaces up to a given Miller index can be unambiguously searched for the lowest-energy termination. By contrast, the construction of explicit interfaces involves many choices, leading to results which may be less reproducible without the exact surface used. Explicit interfaces will also include a lithium chemical potential gradient that is difficult to control or quantify, likely leading to an unknown amount of ionic potential drop mixed with the electronic band alignment. Thus, vacuum alignment is currently the best technique to access $V_{e^-}$.

## S.III. POINT DEFECTS

The formation energy of point defect $X$ in charge state $q$ is given by [4]

$$E^f[X^q] = E_{\text{tot}}[X^q] - E_{\text{tot}}[\text{bulk}] - \sum_i n_i\mu_i + qE_F. \tag{S.10}$$

$E_{\text{tot}}[X^q]$ is the total energy of a supercell containing the defect, $E_{\text{tot}}[\text{bulk}]$ is the total energy of the corresponding bulk cell, $i$ indexes over atomic species added or removed in forming the defect cell, $n_i$ indicates the number of atoms added ($n > 0$) or removed ($n < 0$), and $\mu_i$ is the chemical potential of species $i$. The $\mu_i$ are discussed further in Section [S.V].

The formation energies of the relevant point defects in $LiCoO_2$ as a function of Fermi level are shown in Fig. S.1. Only relevant charge states of the most favorable defects are shown. Further charge states of these defects, the defects $O_{Li}$, $O_{Co}$, $Li_O$, $Co_O$, and an alternative $Li_i$ site were tested and found to be too high in energy to be relevant. The ion-clamped dielectric constant $\varepsilon_r = 44.2$ used for the Freysoldt correction is calculated using PBE+$U$. Defect calculations use a 108-atom cell.

The charge-neutrality Fermi level (taking into account holes present at the VBM, modeled as a parabolic band with a calculated effective mass $m^* = 1.4m_e$) is less than 2 meV below the VBM.

Plots of defect formation energies in LiPON as a function of Fermi level are shown in Fig. S.2. Only relevant charge states of the most favorable defects are shown. Further charge states of these defects, all antisites involving lithium, all native defects involving phosphorus, $O_i$, and various alternative $Li_i$ sites were tested and found to be too high in energy to be relevant. The dielectric constant $\varepsilon_r = 20.6$ for the Freysoldt correction is calculated using PBE. Defect calculations start from a 96-atom supercell. Panel (a) shows the lithium-rich limit ($\mu_{\text{Li}} = 0$ eV), corresponding to the Li/LiPON interface. The dominant defects are positively charged lithium interstitials ($Li_i^+$), neutral oxygen vacancies ($V_O^0$), and negatively charged nitrogen antisites ($N_O^-$). The charge-neutrality Fermi level is 2.36 eV above the valence band. Panel (b) shows the lithium-poor limit ($\mu_{\text{Li}} = -4.02$ eV), corresponding to the LiPON/$LiCoO_2$ interface. The dominant defects are negatively charged lithium vacancies ($V_{\text{Li}}^-$) and positively charged oxygen antisites ($O_N^+$). The charge-neutrality Fermi level is 0.50 eV above the valence band.

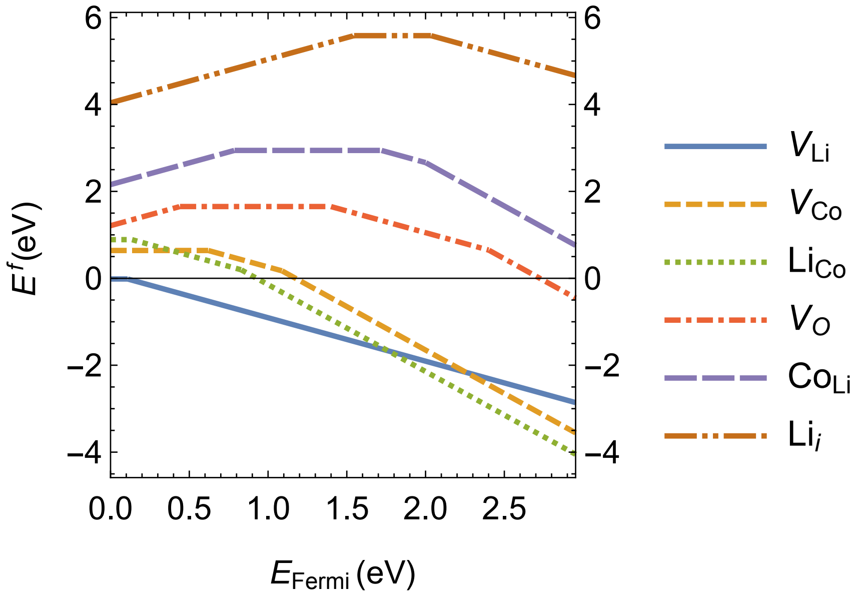


FIG. S.1. Defect formation energy $E^f$ as a function of Fermi level $E_F$ in $LiCoO_2$. Only the lowest stable charge state of each defect is plotted at a given $E_F$. The slope of the line is the charge state of the defect.

## S.IV. BAND STRUCTURES

The band structure of $LiCoO_2$ is shown in Fig. S.3. The band gap is 2.20 eV.

The band structure of *SD*-$Li_2PO_2N$ is shown in Fig. S.4. The band gap is 5.69 eV.

## S.V. CHEMICAL POTENTIALS

For consistency with the $LiCoO_2$ calculations, the bulk phases that go into the Li-Co-O diagram must be calculated using optPBE with $U = 3.32$ uniformly applied to Co $d$ states using the approach of Ref. [5]. The phase diagram is then constructed using PyCDT [6]. The lithium chemical potential is known in the cathode: $\mu_{\mathrm{Li}} = -eV = -4.02$ V. This constrains the other chemical potentials to a region of the phase diagram small enough to be well described by a single point: $\mu_{\mathrm{Co}} = -2.11$ eV and $\mu_{\mathrm{O}} = -2.29$ eV (all chemical potentials are referenced to their respective stable elemental phases).

Since our calculations of LiPON use PBE, Materials Project data [7, 8] may be used to build the phase diagram. The range of $\mu_{\mathrm{Li}}$ is $-0.68$ eV to $-2.64$ eV. The chemical potentials associated with both Li metal and $Li_xCoO_2$ are outside this range. This means interfaces

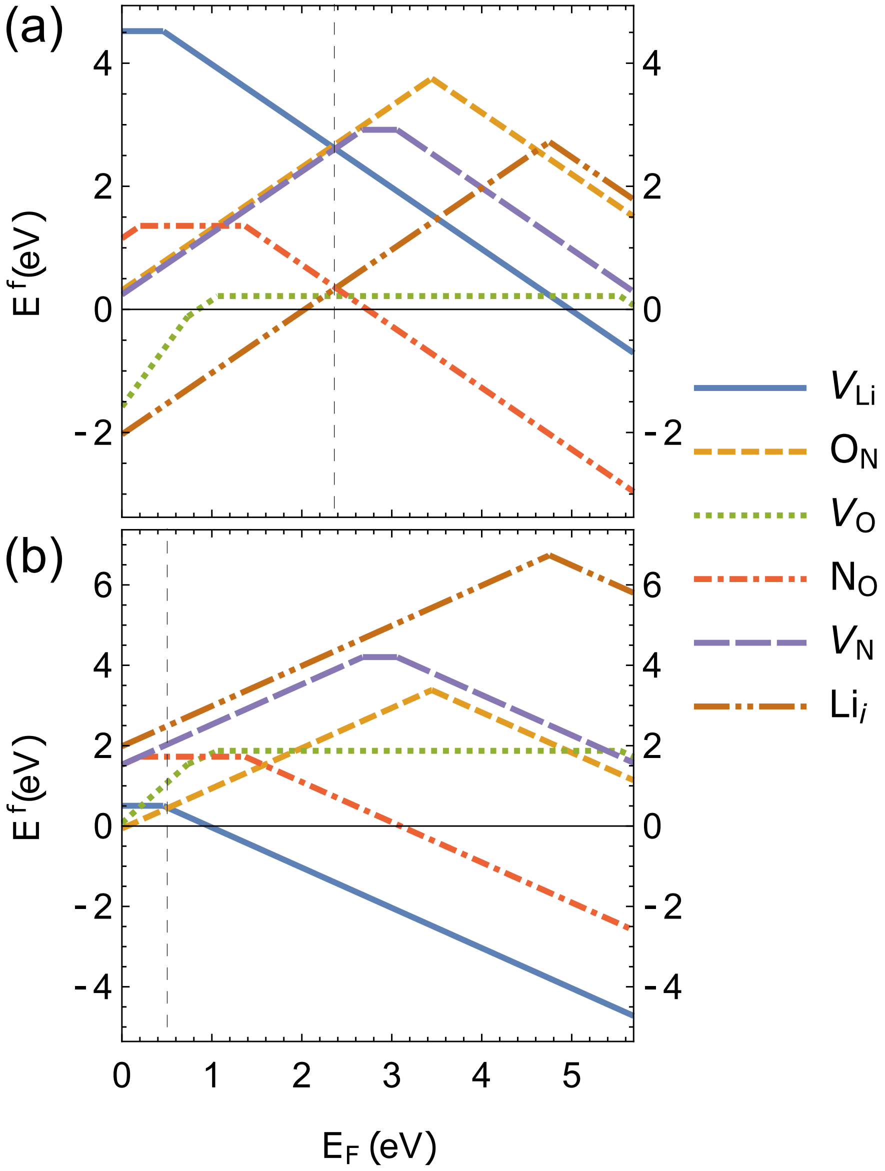


FIG. S.2. Defect formation energies $E^f$ as a function of Fermi level $E_F$ in LiPON. The horizontal axis runs from the VBM ($E_F = 0$ eV) to the CBM ($E_F = 5.69$ eV). The Fermi level determined by charge neutrality at 300K is shown by a dashed vertical line. (a) uses chemical potentials for the Li/LiPON interface, (b) for the LiPON/$LiCoO_2$ interface.

with both cathode and anode are thermodynamically unstable; a globally phase-separated state is more energetically favorable. This is expected, and implications are discussed in the main text. At the lithium-rich limit, chemical potentials for non-Li species are $\mu_{\mathrm{O}} = -4.84$ eV and $\mu_{\mathrm{N}} = -3.12$ eV. At the lithium-poor limit, $\mu_{\mathrm{O}} = -3.20$ eV and $\mu_{\mathrm{N}} = -1.77$ eV.

We now discuss the assumption, used to construct the potential profile in the main text,

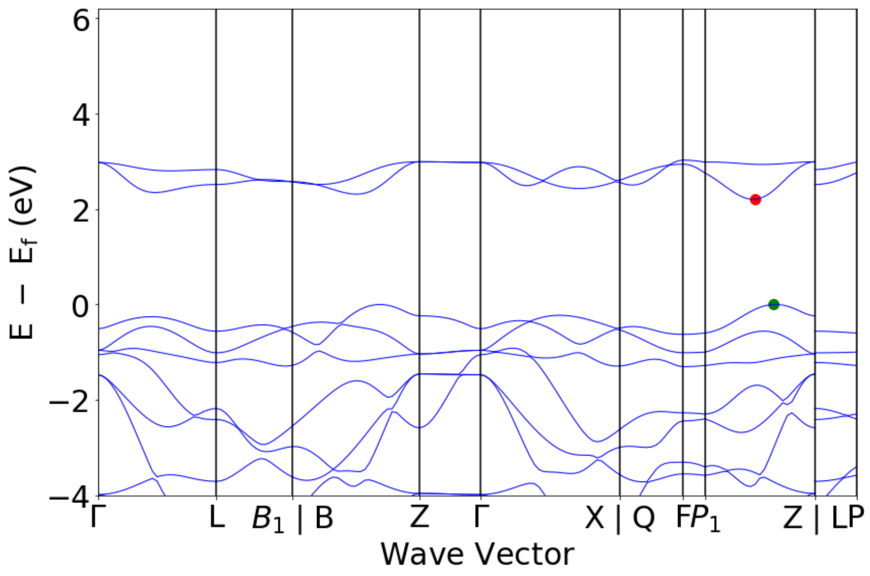


FIG. S.3. Band structure of $LiCoO_2$

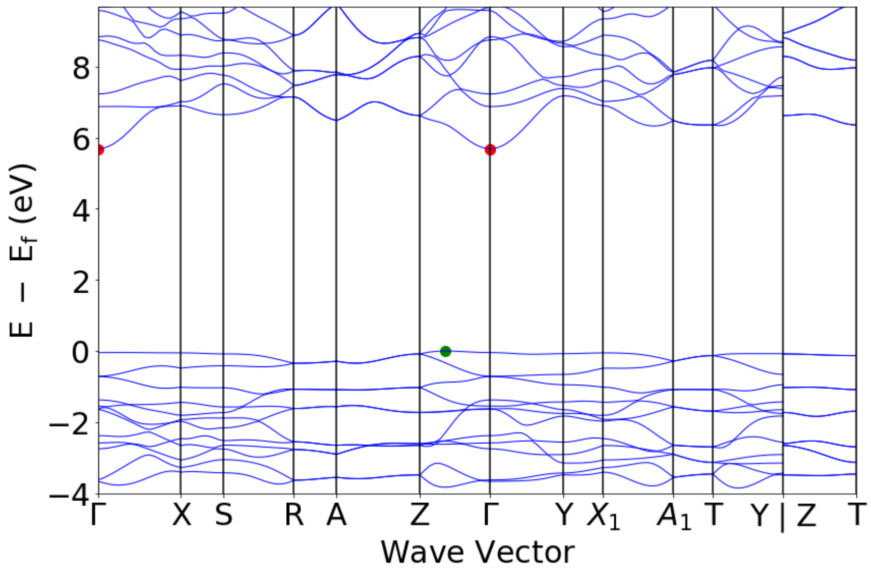


FIG. S.4. Band structure of *SD*-$Li_2PO_2N$

that bulk LiPON near the anode is at the lithium-rich stability limit ($\mu_{\mathrm{Li}} = -0.68$ eV) and near the cathode is at the lithium-poor stability limit ($\mu_{\mathrm{Li}} = -2.64$ eV). This may be considered a "minimum interface" assumption, since it represents the minimum possible potential drop allowed by thermodynamics across each interface. This assumption, while intuitive, may not apply to all devices. Growth, assembly, or operating conditions may constrain the LiPON chemical potentials further than is captured by the first-principles stability window.

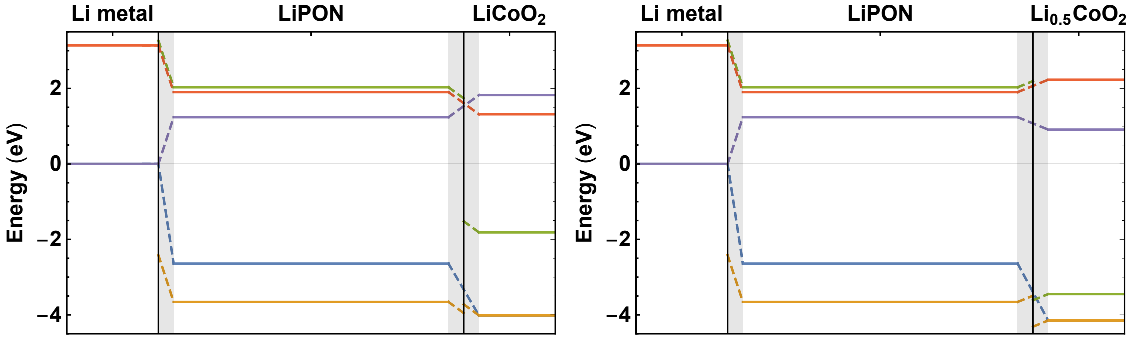


FIG. S.5. SSB potential profiles if LiPON is constrained to its lithium-poor chemical potential limit. By contrast, the profiles in the text use the "minimum-interface assumption", in which the LiPON near the anode is at the lithium-rich limit.

These considerations should be taken into account when comparing the model to a real device, and different chemical potential constraints could lead to quantitative changes in interface dipoles. For example, one could assume that bulk LiPON is at the lithium-poor limit throughout. As shown in Figure S.5, this assumption increases the predicted potential drop at the Li/LiPON interface.

## S.VI. DFT+$U$ AND $U$-RAMPING

As mentioned in the manuscript, Coulomb correlations on the cobalt $d$ states are taken into account through the rotationally-invariant DFT+$U$ approach of Dudarev *et al* [5]. A value of $U = 3.32$ eV is standard [9] and has been shown to give good results in combination with "opt"-type functionals used to capture van der Waals interactions [10]. As described by Aykol *et al.* [10], we find that this method is quite sensitive to initial conditions of the magnetic moments of cobalt and can easily converge to solutions which are unstable yet self-consistent at the Kohn-Sham level. We attempted various methods to deal with this sensitivity to initial conditions, and found a $U$-ramping procedure [11] to work best. Much as described in Ref. [10], we found this procedure to reliably give very low-energy electronic configurations.

## S.VII. FERMI LEVEL CLARIFICATION

The term “Fermi level” is often used to refer to the chemical potential of electrons referenced to the VBM of the host crystal. In the manuscript, this usage has been denoted $E_F$, following standard point defect formalism. We also use the term “Fermi level” to refer to the electrochemical potential of electrons. Unlike $E_F$, this may be compared across different materials and includes effects of the electrostatic potential. We denote this usage $\tilde{\mu}_{e^-}$ and choose lithium metal as the zero reference.

Conversion between the two different notions of “Fermi level” may be accomplished by the equation

$$\tilde{\mu}_{e^-} = E_F - I_{\text{host}} + \psi_{\text{Li}} - e\phi \ . \tag{S.11}$$

The term $-I_{\text{host}} + \psi_{\text{Li}}$ converts the reference from the host valence band to lithium metal and $-e\phi$ adjusts for shifts in the local vacuum level due to the electrostatic potential $\phi$.

## S.VIII. CODES AND DATA

Raw DFT data and code modeling the potential profile are available upon request from the corresponding author Yue Qi: yueqi@egr.msu.edu.

---


[1] S. P. Ong, W. D. Richards, A. Jain, G. Hautier, M. Kocher, S. Cholia, D. Gunter, V. L. Chevrier, K. A. Persson, and G. Ceder, Comput. Mater. Sci **68**, 314 (2013).

[2] P. G. Moses, M. Miao, Q. Yan, and C. G. Van de Walle, J. Chem. Phys. **134**, 084703 (2011).

[3] C. G. Van de Walle and R. M. Martin, Phys. Rev. B **35**, 8154 (1987).

[4] C. Freysoldt, B. Grabowski, T. Hickel, J. Neugebauer, G. Kresse, A. Janotti, and C. G. Van de Walle, Rev. Mod. Phys. **86**, 253 (2014).

[5] S. L. Dudarev, G. A. Botton, S. Y. Savrasov, C. J. Humphreys, and A. P. Sutton, Phys. Rev. B **57**, 1505 (1998).

[6] D. Broberg, B. Medasani, N. E. Zimmermann, G. Yu, A. Canning, M. Haranczyk, M. Asta, and G. Hautier, Comput. Phys. Commun **226**, 165 (2018).

[7] A. Jain, S. P. Ong, G. Hautier, W. Chen, W. D. Richards, S. Dacek, S. Cholia, D. Gunter, D. Skinner, G. Ceder, and K. A. Persson, APL Mater. **1**, 011002 (2013).

[8] S. P. Ong, S. Cholia, A. Jain, M. Brafman, D. Gunter, G. Ceder, and K. A. Persson, Comput. Mater. Sci **97**, 209 (2015).

[9] L. Wang, T. Maxisch, and G. Ceder, Phys. Rev. B **73**, 195107 (2006).

[10] M. Aykol, S. Kim, and C. Wolverton, J. Phys. Chem. C **119**, 19053 (2015).

[11] B. Meredig, A. Thompson, H. A. Hansen, C. Wolverton, and A. van de Walle, Phys. Rev. B **82**, 195128 (2010).
